# Supplementary material for: Learned Lock-free Search Data Structures
Source: arXiv:2308.11205 source file (2023-08-22)
Supplement: Supplementary file 1 [file appendix.tex]

As mentioned in Section \ref{sec:lfmodel} we documented the cardinality of the hierarchy or the total number of comparison-based or model-based nodes formed in each technique shown in Table \ref{table:nodes}. Because a single linear model may approximate a very large data array with an error constraint, the learnt data structure can handle enormously large nodes which leads to considerably lower hierarchy than concurrent classical ones. This less number of nodes gives an added advantage to \kan that due to its number of nodes, the traversal time becomes less, and there is no need to rebalance the structure as compared to its classical tree counterparts.

As already discussed in Section \ref{sec:lfmodel} we have tried different regression fitting models for \kan. Regression Error and the time taken for the same can be seen in Table \ref{table:collect}. As discussed earlier Lock-Free approach has taken the least time when compared to others as there is no need for synchronization.
\input{table/Modelcount}

Table \ref{time} shows the time required to construct the structures based on various indices. We can observe that the single-pass model-based learning indexes require much less time to create the search structure.
Conventional tree structures, such as (a, b)-tree and C-IST, generate a huge number of nodes and have a long indexing time. C-IST must calculate the parameters for interpolation search every time it rebalances, which becomes more time-consuming as the amount of data items grows. This explains why learnt index systems perform better in terms of memory and time. Furthermore, single-pass procedures provide the greatest number of models while taking the least amount of time to prepare the model.
% Please add the following required packages to your document preamble:
% \usepackage{multirow}
% \usepackage{graphicx}
\begin{table}[]
\caption{Time taken for building the structure}
\label{time}
\resizebox{\columnwidth}{!}{%
\begin{tabular}{|cc|c|c|c|c|c|c|}
\hline
\multicolumn{2}{|l|}{Workloads}                         & books   & fb  & osmc & normal & log normal & uniform\_sparse \\ \hline
\multicolumn{2}{|l|}{Number of Data} & 200M    & 200M    & 200M  & 200M  & 200M    & 200M  \\ \hline
\multicolumn{1}{|l|}{\multirow{4}{*}{Time}} & LPA & 92.1056 & 105 & 98.9 & 100.9  & 117.1      & 83.7            \\ \cline{2-8} 
\multicolumn{1}{|l|}{}   & PGM       & 41.4    & 56      & 53.2  & 64.4  & 64.4    & 38.4  \\ \cline{2-8} 
\multicolumn{1}{|l|}{}   & (a,b)-tree   & 278.4   & 277.2   & 273.9 & 273.2 & 278.3   & 274.7 \\ \cline{2-8} 
\multicolumn{1}{|l|}{}   & C-IST      & 45406.4 & 42532.9 &  48895.5     &  46243.1     & 45751.1 &   48215.1    \\ \hline
\end{tabular}%
}
\end{table}
